# Supplementary material for: Learning Human-Human Interactions in Images from Weak Textual Supervision
Source: arXiv:2304.14104 source file (2023-09-18)
Supplement: Supplementary file 2 [file supp-1-02-imsitu-8beams.tex]

\subsection{Results on \imsituhhi for top 8 beams} \label{sec:imsitu_8beams}

See Table \ref{tab:imsitu_results_8beams} for additional results on the \imsituhhi dataset when using the top 5 and 8 beams (via beam search with 32 beams) for relevant models.

\begin{table*}[t]
  \centering
  \setlength{\tabcolsep}{3.5pt}
  
  \begin{tabularx}{1.0\textwidth}{llccccccccccccccccc}
     & &
    {\small \rotatebox[origin=l]{90}{\textbf{Average sim.}}} &
    &
    {\small\rotatebox[origin=l]{90}{socializing}} & {\small\rotatebox[origin=l]{90}{distributing} }& {\small\rotatebox[origin=l]{90}{teaching}} & {\small\rotatebox[origin=l]{90}{communicating}} & {\small\rotatebox[origin=l]{90}{interviewing}} & {\small\rotatebox[origin=l]{90}{lecturing}} &
    {\small\rotatebox[origin=l]{90}{training}} &
    {\small\rotatebox[origin=l]{90}{providing}} &
    {\small\rotatebox[origin=l]{90}{instructing}} &
    {\small\rotatebox[origin=l]{90}{giving}} &
    {\small\rotatebox[origin=l]{90}{pushing}} &
    {\small\rotatebox[origin=l]{90}{helping}} &
    {\small\rotatebox[origin=l]{90}{asking}} &
    {\small\rotatebox[origin=l]{90}{coaching}} &
    {\small\rotatebox[origin=l]{90}{talking}} \\
    \midrule
    \textbf{Results@5} \\
    ENv2 & COCO & 0.26 &  & 0.21 & 0.10 & 0.26 & 0.23 & 0.30 & 0.21 & 0.27 & 0.31 & 0.13 & 0.49 & 0.45 & 0.35 & 0.49 & 0.33 & 0.31 \\% & 0.59 & 0.16 & 0.33 & 0.24 \\
    CLIPCap & COCO  & 0.25 &  & 0.19 & 0.09 & 0.29 & 0.26 & 0.31 & 0.20 & 0.27 & 0.26 & 0.12 & 0.47 & 0.41 & 0.29 & 0.48 & 0.32 & 0.66 \\% & 0.30 & 0.17 & 0.38 & 0.22 \\
    CLIPCap & CC  & 0.35 &  & 0.21 & 0.30 & 0.48 & 0.33 & 0.28 & 0.31 & 0.37 & 0.43 & 0.21 & 0.56 & 0.42 & 0.48 & 0.47 & 0.31 & 0.64 \\% & 0.55 & 0.32 & 0.58 & 0.35 \\
    CLIPCap & CC+WW & 0.18  &  & 0.05 & 0.15 & 0.22 & 0.14 & \textbf{0.60} & 0.16 & 0.17 & 0.22 & 0.11 & 0.46 & 0.15 & 0.21 & 0.22 & 0.15 & 0.24 \\% & 0.13 & 0.11 & 0.17 & 0.26\\
    EncDec &pHHI & \underline{0.40} &  & \textbf{0.30} & \textbf{0.35} & \underline{0.49} & \underline{0.41} & 0.39 & \underline{0.33} & \underline{0.51} & \underline{0.51} & \underline{0.23} & \underline{0.79} & \underline{0.47} & \underline{0.49} & \underline{0.57} & \textbf{0.92} & \underline{0.86} \\% & 0.42 & 0.35 & 0.47 & 0.58 \\
    CLIPCap & CC+pHHI & \textbf{0.44} &  & \underline{0.29} & \textbf{0.35} & \textbf{0.85} & \textbf{0.44} & \underline{0.41} & \textbf{0.40} & \textbf{0.56} & \textbf{0.56} & \textbf{0.27} & \textbf{0.88} & \textbf{0.48} & \textbf{0.56} & \textbf{0.58} & \underline{0.86} & \textbf{0.92} \\% & 0.40 & 0.42 & 0.45 & 0.63 \\
    \midrule
    \textbf{Results@8} \\
    ENv2 & COCO & 0.28 &  & 0.22 & 0.12 & 0.27 & 0.24 & 0.30 & 0.21 & 0.28 & 0.32 & 0.13 & 0.51 & 0.47 & 0.37 & 0.50 & 0.35 & 0.34 \\% & 0.61 & 0.17 & 0.38 & 0.25 \\
    CLIPCap & COCO  & 0.26 &  & 0.20 & 0.10 & 0.31 & 0.27 & 0.31 & 0.21 & 0.28 & 0.26 & 0.12 & 0.48 & 0.43 & 0.31 & 0.49 & 0.32 & 0.67 \\% & 0.31 & 0.18 & 0.39 & 0.23 \\
    CLIPCap & CC  & 0.37 &  & 0.23 & 0.31 & 0.51 & 0.34 & 0.31 & 0.32 & 0.40 & 0.45 & 0.22 & 0.59 & 0.45 & 0.51 & 0.49 & 0.32 & 0.70 \\% & 0.60 & 0.33 & 0.61 & 0.3 \\
    CLIPCap & CC+WW & 0.21 &  & 0.06 & 0.16 & 0.25 & 0.16 & \textbf{0.62} & 0.16 & 0.20 & 0.24 & 0.12 & 0.51 & 0.20 & 0.23 & 0.26 & 0.18 & 0.32 \\% & 0.16 & 0.13 & 0.20 & 0.28 \\
    EncDec & pHHI & \underline{0.44} &  & \textbf{0.33} & \textbf{0.38} & \underline{0.55} & \underline{0.44} & \underline{0.42} & \underline{0.34} & \underline{0.54} & \underline{0.56} & \underline{0.25} & \underline{0.85} & \underline{0.49} & \underline{0.56} & \underline{0.59} & \textbf{0.94} & \underline{0.91} \\% & 0.44 & 0.38 & 0.49 & 0.65 \\
    CLIPCap & CC+pHHI & \textbf{0.47} &  & \textbf{0.33} & \underline{0.37} & \textbf{0.90} & \textbf{0.46} & 0.41 & \textbf{0.43} & \textbf{0.60} & \textbf{0.59} & \textbf{0.29} & \textbf{0.92} & \textbf{0.50} & \textbf{0.59} & \textbf{0.61} & \underline{0.91} & \textbf{0.96} \\% & 0.43 & 0.45 & 0.48 & 0.74 \\
    \bottomrule
  \end{tabularx}
  \vspace{0pt}
  \caption{Results on \textbf{\imsituhhi} for top 5 and 8 beams, as described in Section \ref{sec:imsitu_8beams}.}
\label{tab:imsitu_results_8beams}
\end{table*}
