# Supplementary material for: Learning Human-Human Interactions in Images from Weak Textual Supervision
Source: arXiv:2304.14104 source file (2023-09-18)
Supplement: Supplementary file 4 [file supp_wenda_results.tex]

\begin{table*}[t]
  \centering
  \setlength{\tabcolsep}{5.5pt}
  
  \begin{tabularx}{0.96\textwidth}{llccccccccccccc}
    \toprule
    & &
    \multicolumn{4}{c}{\textbf{WW}} &
    \multicolumn{4}{c}{\textbf{CC}} &
    \multicolumn{4}{c}{\textbf{COCO}}
    \\
    \cmidrule(lr){3-6}
    \cmidrule(lr){7-10}
    \cmidrule(lr){11-14}
    Method & Training Data & BL$\,\uparrow$ & $p_e \uparrow$ & $p_c \downarrow$ & sim$\,\uparrow$ & BL$\,\uparrow$ & $p_e \uparrow$ & $p_c \downarrow$ & sim$\,\uparrow$ & BL$\,\uparrow$ & $p_e \uparrow$ & $p_c \downarrow$ & sim$\,\uparrow$  \\
    \midrule
\textbf{Results@8} \\
Env2 & COCO & 0.29 & 0.34 & 0.15 & 0.42 & 0.31 & 0.35 & 0.25 & 0.48 & 0.36 & 0.59 & 0.10 & 0.53 \\
Env2 & COCO & 0.32 & 0.53 & 0.18 & 0.43 & 0.30 & 0.41 & 0.25 & 0.47 & 0.35 & 0.55 & 0.21 & 0.50 \\
CLIPCap & CC & 0.38 & 0.47 & 0.17 & 0.48 & 0.32 & 0.35 & 0.19 & 0.53 & 0.34 & 0.26 & 0.11 & 0.45 \\
CLIPCap & CC+WW & 0.34 & 0.22 & 0.48 & 0.35 & 0.36 & 0.42 & 0.10 & 0.33 & 0.35 & 0.34 & 0.06 & 0.25 \\
EncDec & pHHI & \textbf{0.60} & \underline{0.69} & \textbf{0.06} & \textbf{0.69} & \underline{0.55} & \underline{0.72} & \underline{0.05} & \underline{0.64} & \underline{0.50} & \underline{0.66} & \underline{0.04} & \underline{0.61} \\
CLIPCap & CC+pHHI & \textbf{0.60} & \textbf{0.70} & \underline{0.07} & \underline{0.68} & \textbf{0.63} & \textbf{0.81} & \textbf{0.03} &  \textbf{0.72} & \textbf{0.55} & \textbf{0.78} & \textbf{0.03} & \textbf{0.67} \\
    \bottomrule
  \end{tabularx}
  \vspace{5pt}
  \caption{Top-8 results on \textbf{\datasetname{}} split by data source -- Who's Waldo (WW), Conceptual Captions (CC), and COCO Captions -- as described in Section \ref{sec:supp_wenda_source}.}
\label{tab:supp_wenda_results}
\end{table*}
